# Supplementary material for: Simultaneous detection and estimation of trait associations with genomic phenotypes
Source: arXiv:1611.04473 source file (2016-11-14)
Supplement: Supplementary file 1 [file jade_supp.pdf]

# Simultaneous detection and estimation of trait associations with genomic phenotypes — Supplementary Materials

Jean Morrison\* <sup>†</sup>, Noah Simon<sup>†</sup>, Daniela Witten<sup>‡</sup>

<sup>†</sup> *Department of Biostatistics*

<sup>‡</sup> *Departments of Statistics and Biostatistics*

*University of Washington, Seattle WA, 98195, USA*

jeanm5@uw.edu

## A. TREND FILTERING

$\mathbf{D}^{k+1,s}$  in (2.2) is the discrete  $(k+1)$ st derivative operator for sites  $\mathbf{s} = (s_1, \dots, s_p)$ . This matrix can be defined recursively. For  $k = 0$ ,

$$\mathbf{D}^{1,s} \equiv \mathbf{D}^1 = \begin{pmatrix} -1 & 1 & 0 & \cdots & 0 & 0 \\ 0 & -1 & 1 & \cdots & 0 & 0 \\ \vdots & \vdots & \vdots & \ddots & \vdots & \vdots \\ 0 & 0 & 0 & \cdots & -1 & 1 \end{pmatrix}, \quad (\text{A.1})$$

a  $(p-1) \times p$  matrix that does not actually depend on  $\mathbf{s}$ . This corresponds exactly to the fused lasso (Tibshirani *and others*, 2005). For  $k \geq 1$ ,

$$\mathbf{D}^{k+1,s} = \mathbf{D}^1 \cdot \text{diag} \left( \frac{k}{s_{k+1} - s_1} \cdots \frac{k}{s_p - s_{p-k}} \right) \cdot \mathbf{D}^{k,s} \equiv \mathbf{D}^1 \tilde{\mathbf{D}}^{k,s} \quad (\text{A.2})$$

as described in Ramdas and Tibshirani (2015) and Tibshirani (2014). Equation A.2 admits a slight abuse of notation:  $\mathbf{D}^1$  in (A.2) is the  $(p-k-1) \times (p-k)$ -dimensional version of (A.1).

\*To whom correspondence should be addressed.

## B. DETAILS OF ALGORITHM 1

## B.1 Step 3(iii)

When  $M = 2$ , the  $\beta_1$  and  $\beta_2$  updates have a simple closed form, given in [Danaher and others \(2014\)](#):

$$\begin{aligned}\eta_1 &= \text{sign}(\mathbf{z}_1 - \mathbf{z}_2) \cdot \max\left(\left|\frac{\mathbf{z}_1 - \mathbf{z}_2}{2}\right| - \frac{\gamma}{\rho_\beta}, 0\right), & \eta_2 &= \frac{\mathbf{z}_1 + \mathbf{z}_2}{2}, \\ \beta_1 &= \eta_1 + \eta_2, & \beta_2 &= \eta_2 - \eta_1,\end{aligned}$$

where  $\mathbf{z}_m = \boldsymbol{\theta}_m + \mathbf{u}_m^{(\beta)}$ . Here, the sign and max operators are applied element-wise.

## B.2 Step Size and Stopping Criteria

Step size update rules and stopping criteria are taken from [Boyd and others \(2010\)](#). The rules are based on primal and dual residuals, defined as

$$\begin{aligned}\mathbf{r}_{\text{primal}}^{(\alpha m)} &= \tilde{\mathbf{D}}^{k,s} \boldsymbol{\theta}_m - \boldsymbol{\alpha}_m, & \mathbf{r}_{\text{primal}}^{(\beta)} &= \boldsymbol{\beta} - \boldsymbol{\theta}, \\ \mathbf{r}_{\text{dual}}^{(\alpha m)} &= \rho_{\alpha m}^{old} \left[ \tilde{\mathbf{D}}^{k,s} \right]^\top (\boldsymbol{\alpha}_m - \boldsymbol{\alpha}_m^{old}), & \mathbf{r}_{\text{dual}}^{(\beta)} &= \rho_\beta^{old} (\boldsymbol{\beta} - \boldsymbol{\beta}^{old}),\end{aligned}$$

where  $\boldsymbol{\alpha}^{old}$ ,  $\boldsymbol{\beta}^{old}$ , and  $\rho^{old}$  are the  $\boldsymbol{\alpha}$ ,  $\boldsymbol{\beta}$ , and  $\rho$  values from the previous iteration of the algorithm.

For the first 500 iterations of the ADMM algorithm, we update the step sizes as

$$\rho_* = \begin{cases} \tau_{\text{incr}} \rho_*^{old} & \left\| \mathbf{r}_{\text{primal}}^* \right\|_2 > \mu \left\| \mathbf{r}_{\text{dual}}^* \right\|_2 \\ \rho_*^{old} / \tau_{\text{decr}} & \left\| \mathbf{r}_{\text{dual}}^* \right\|_2 > \mu \left\| \mathbf{r}_{\text{primal}}^* \right\|_2 \\ \rho_*^{old} & \text{otherwise} \end{cases},$$

where  $*$  indicates the  $m+1$  indices  $\alpha_1, \dots, \alpha_M$  and  $\beta$ ;  $\rho_*^{old}$  indicates the step size at the previous iteration; and  $\tau_{\text{incr}}$ ,  $\tau_{\text{decr}}$  and  $\mu$  are parameters which we set to 2, 2 and 10 as suggested by [Boyd and others \(2010\)](#). We initialize  $\rho_\beta = 1$  and  $\rho_{\alpha m} = \lambda \left( \frac{\max(\{s_j\}) - \min(\{s_j\})}{p} \right)^{k-1}$  based on a suggestion in [Ramdas and Tibshirani \(2015\)](#).

We use the stopping criteria discussed in Section 3.3.1 of [Boyd and others \(2010\)](#), terminating

when

$$\begin{aligned}\|\mathbf{r}_{\text{primal}}\|_2 &\leq \epsilon^{\text{abs}} \sqrt{M(2p-k)} + \epsilon^{\text{rel}} \max \left( \sqrt{\sum_m \left[ \|\tilde{\mathbf{D}}^{k,s} \boldsymbol{\theta}_m\|_2^2 + \|\boldsymbol{\theta}_m\|_2^2 \right]}, \sqrt{\sum_m \left[ \|\boldsymbol{\alpha}_m\|_2^2 + \|\boldsymbol{\beta}_m\|_2^2 \right]} \right), \\ \|\mathbf{r}_{\text{dual}}\|_2 &\leq \epsilon^{\text{abs}} \sqrt{M(2p-k+1)} + \epsilon^{\text{rel}} \left( \sqrt{\|\tilde{\mathbf{D}}^{k,s} \mathbf{u}_m^{(\alpha)}\|_2^2 + \|\mathbf{u}_m^{(\beta)}\|_2^2} \right),\end{aligned}$$

where  $\mathbf{r}_{\text{primal}} = (\mathbf{r}_{\text{primal}}^{(\alpha 1)}, \dots, \mathbf{r}_{\text{primal}}^{(\alpha M)}, \mathbf{r}_{\text{primal}}^{(\beta)})$ ,  $\mathbf{r}_{\text{dual}} = (\mathbf{r}_{\text{dual}}^{(\alpha 1)}, \dots, \mathbf{r}_{\text{dual}}^{(\alpha M)}, \mathbf{r}_{\text{dual}}^{(\beta)})$ , and  $\epsilon^{\text{abs}}$  and  $\epsilon^{\text{rel}}$  are parameters which, by default, we set to  $10^{-4}$  and  $10^{-8}$ .

### C. CROSS-VALIDATION OF $\gamma$

The JADE optimization problem given in (2.4) has an equivalent constrained form,

$$\begin{aligned}\underset{\boldsymbol{\theta}_1, \dots, \boldsymbol{\theta}_M}{\text{minimize}} \quad & \sum_{m=1}^M \frac{N_m}{2} \|\mathbf{A}_m(\bar{\mathbf{y}}_m - \boldsymbol{\theta}_m)\|_2^2 + \lambda \sum_{m=1}^M \|\mathbf{D}^{k+1,s} \boldsymbol{\theta}_m\|_1 \\ \text{subject to} \quad & \sum_{m < m'} \|\boldsymbol{\theta}_m - \boldsymbol{\theta}_{m'}\|_1 \leq C_\gamma.\end{aligned}\tag{C.3}$$

For each  $\gamma$ , there is a corresponding  $C_\gamma$  such that (2.4) and (C.3) have identical solutions. The mapping from  $\gamma$  to  $C_\gamma$  is quite complicated, and depends on the data. In practice, we have seen that solutions to (C.3) for a fixed value of  $C_\gamma$  are more similar across cross-validation folds than solutions to (2.4) for a fixed  $\gamma$ , so we choose to cross-validate based on  $C_\gamma$  rather than  $\gamma$ .

Unfortunately, it is difficult to solve (C.3) for a specified value of  $C_\gamma$ . Instead, we choose a grid of  $C_\gamma$  values, and in each fold of our cross-validation we find a grid of  $\gamma$  values that approximately covers those  $C_\gamma$  values. We then linearly interpolate to estimate test error for our specified grid of  $C_\gamma$  values.

## D. DETAILS OF FIGURES 3, 4, AND 5 IN SECTION 4 OF MAIN MANUSCRIPT

D.1 *Calculation of curves*

For the  $t$ -statistic methods, we allowed the significance threshold (the absolute value threshold at which a statistic is declared significant) to vary between 0 and the value of the largest statistic observed. For a given threshold value, and for a given simulated data set, we computed the true and false positive rates (TPR and FPR) using information about whether each site is part of a differential region. For a given simulated data set, we then linearly interpolated the corresponding TPR and FPR values. Finally, for each FPR value along a fine grid, we averaged the corresponding TPR values across the simulated data sets, in order to obtain the curves displayed in the figure.

For JADE, we varied the value of  $\gamma$  in (2.4). For each value of  $\gamma$ , and for a given simulated data set, we computed the TPR and the FPR of the corresponding JADE fit. For a given simulated data set, we then linearly interpolated the corresponding TPR and FPR values. Finally, for each FPR value along a fine grid, we averaged the corresponding TPR values across the simulated data sets, in order to obtain the curve displayed in the figure.

D.2 *Calculation of colored points*

For the  $t$ -statistic methods, for each simulated data set, we calculated the value of the significance threshold that resulted in an estimated false discovery rate of 10%, and calculated the TPR and FPR corresponding to this threshold. We then averaged these TPRs and FPRs over the simulated data sets, and displayed the resulting average FPR and average TPR using a colored point.

For JADE, for each simulated data set, we used cross-validation to select a value for  $\gamma$ , and calculated the corresponding TPR and FPR. We then averaged these TPRs and FPRs over the simulated data sets, and displayed the resulting average TPR and average FPR using a colored point.

## E. ADDITIONAL SIMULATION RESULTS

### E.1 Variable Sample Size

In Section 4 of the main paper, we present simulations using  $M = 2$  groups of size  $n_1 = n_2 = 10$ . In practice, due to time and cost constraints, experiments tend to have small sample sizes. For example, the ENCODE project provides DNA methylation and more for a large number of cell types, with only one biological replicate for most cell types.

In this section, we explore the effect of sample size in the context of the normal simulations described in Section 4.1.

We considered two simulation settings:

Setting (i): We generated data as in (4.7) of the main manuscript, with  $\epsilon_{imj} \sim N(0, 0.4 \cdot n_m)$ .

Setting (ii): We generated data according to (4.7) and (4.8) of the main manuscript, with  $\sigma^2$  and  $\sigma_{\text{re}}^2$  chosen so that  $\sigma^2 + \sigma_{\text{re}}^2 = 0.5 \cdot n_m$  and  $\sigma_{\text{re}}^2 / (\sigma^2 + \sigma_{\text{re}}^2) = 0.2$ .

In each simulation setting, we generated data with  $n_1 = n_2$  equal to 3, 5, 10, 20, and 50. Results are shown in Supplementary Figure 1. Using a larger sample size has little effect on JADE, but results in slightly higher power for the  $t$ -test methods.

### E.2 Region-Level Results

In Section 4 of the main paper, we investigate the site-level accuracy of JADE and the other methods. In this section, we instead perform a region-level analysis.

We treat consecutive sites within a differential region detected by JADE as a single discovery. For the  $t$ -statistic approaches, for a given threshold value, we define a discovery to be any string of three or more consecutive sites for which the  $t$ -statistic exceeds that threshold in absolute value. Discoveries separated by only one non-significant site are merged.

We define a true positive to be any discovery that overlaps a signal region, and a false positive

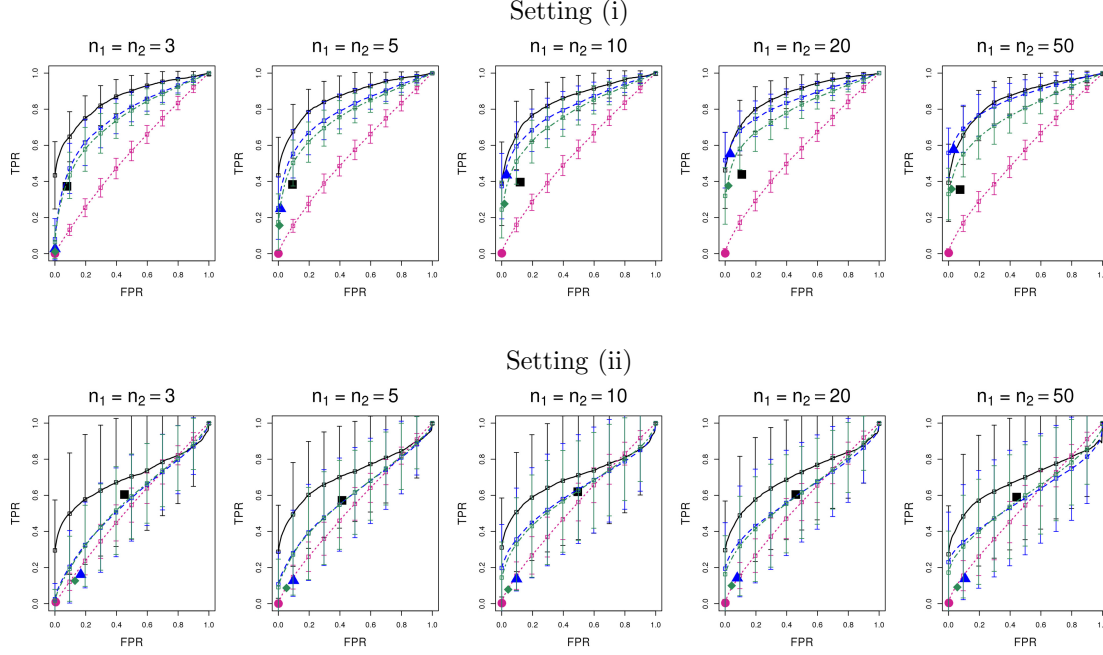

Fig. 1: Simulation study described in Section E.1. Curves display the average TPR for a fixed FPR, averaged over 100 simulations. The vertical bars indicate one sample standard deviation. Points indicate average TPR and FPR achieved for JADE with the tuning parameter selected by cross-validation, and for the  $t$ -test approaches with an FDR threshold of 10%. Methods shown are JADE (—, ■), per-site  $t$ -tests applied to the raw data (---, ●), and per-site  $t$ -tests after smoothing the raw data using splines (---, ▲) and local likelihood (---, ◆).

to be any discovery that does not overlap a signal region. The TPR is defined to be the proportion of signal regions that overlap a discovery. This means that a method that makes multiple disjoint discoveries within one large signal region will be assigned the same TPR as a method that make a single discovery that exactly overlaps the signal region.

In this region-level analysis, it is hard to define the FPR, since there is no natural partition of non-signal sites into regions. Therefore, instead of considering the FPR, we simply consider the number of false positives.

These definitions of TPR and false positives are sensible when the discoveries span small regions. If, however, a method produces a few discoveries that span long regions containing most of the sites, then the method will have a high TPR and few false positives but qualitatively

undesirable results. To avoid this problem, we limit our analysis to a range of thresholds for the t-statistic methods and  $\gamma$  values for JADE that result in discoveries that span less than 50% of the total region. Furthermore, we note that both site-level and region-level results should be considered when summarizing a method’s accuracy.

Region-level summaries for the simulations presented in Figures 3, 4, 5 of the main text are shown in Supplementary Figures 2, 3, and 4. Additional details of how these figures were generated are provided in Section D, with FPR replaced with the number of false positives. The figures indicate that all methods perform very well in terms of region-level metrics, with the exception of methylKit in the binomial simulations shown in Supplementary Figure 4.

In order to see more differences between the methods, we devised a more challenging setting, in which the data are generated using the mean profiles in Supplementary Figure 5 rather than in Figure 2 of the main text. We generated data under the auto-regressive model of Section 4.1.1, with  $p = 500$ ,  $\sigma = 2$ , and  $\rho \in \{0, 0.2, 0.4\}$ . The results are shown in Supplementary Figure 6. For a given number of false positives, JADE has a slightly higher TPR than competing methods.

## F. READ TILING IN BINOMIAL SIMULATIONS

We now describe the strategy used to generate  $n_{imj}$  in Section 4.2. In order to mimic the variable read depth observed in methylation sequencing data, reads at each position are assigned by layering contiguous tiles. A schematic of 30 tiles is shown in Supplementary Figure 7. A tile is placed by sampling a length from an  $\text{Exponential}(30)$  distribution, and a start point from a  $\text{Uniform}(-30, 300)$  distribution. Portions of tiles extending above 300 or below 1 are discarded. For each observation, 110 tiles are placed initially, so that in expectation there are 10 reads per site. For each site that has zero reads at the end of this procedure, one additional tile is drawn using the sampling scheme above, conditional on covering the zero-read site. This procedure guarantees that every site is covered, while keeping the expected coverage of each site close to 10 reads.

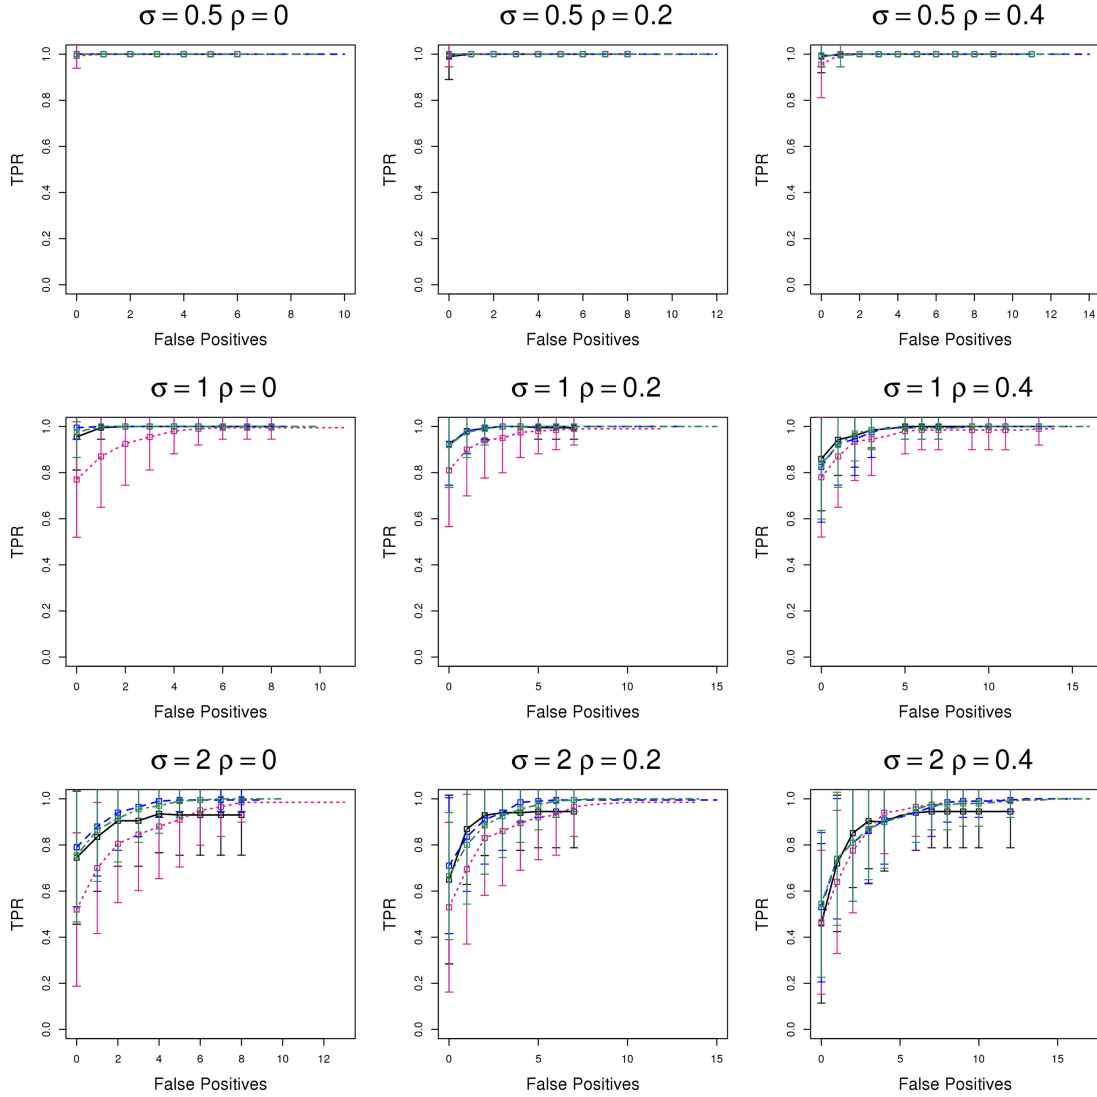

Fig. 2: Performance of JADE and competing methods in the normal autoregressive simulations presented in Figure 3 of the main text. Here, performance is quantified using a region-level analysis, described in Section E.2. Curves display the average region-level TPR, for a fixed number of false positives. The vertical bars indicate one sample standard deviation. Methods shown are JADE (—), per-site  $t$ -tests applied to the raw data (···), and per-site  $t$ -tests after smoothing the raw data using splines (— —) and local likelihood (— · —).

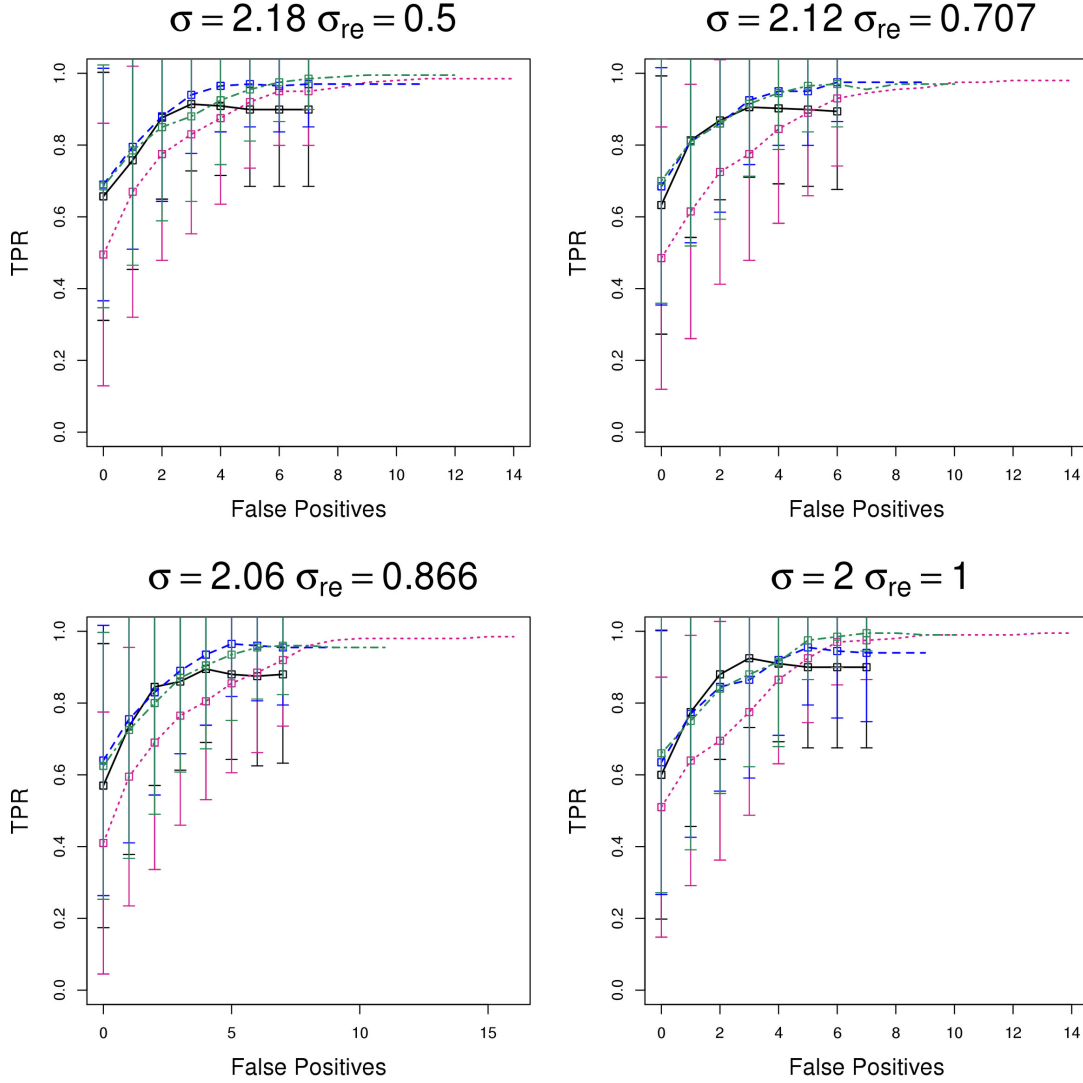

Fig. 3: Performance of JADE and competing methods in the normal random effects simulations presented in Figure 4 of the main text. Here, performance is quantified using a region-level analysis, described in Section E.2. Details are as in Supplementary Figure 2.

## G. ADDITIONAL RESULTS FOR METHYLATION ANALYSIS OF SECTION 5

### G.1 *Loss-of-Methylation Over the Course of Muscle Cell Development*

It is well-established in the literature that as myoblasts develop into mature skeletal muscles, a loss of methylation tends to occur (Hupkes *and others*, 2011; Segalés *and others*, 2014; Palacios

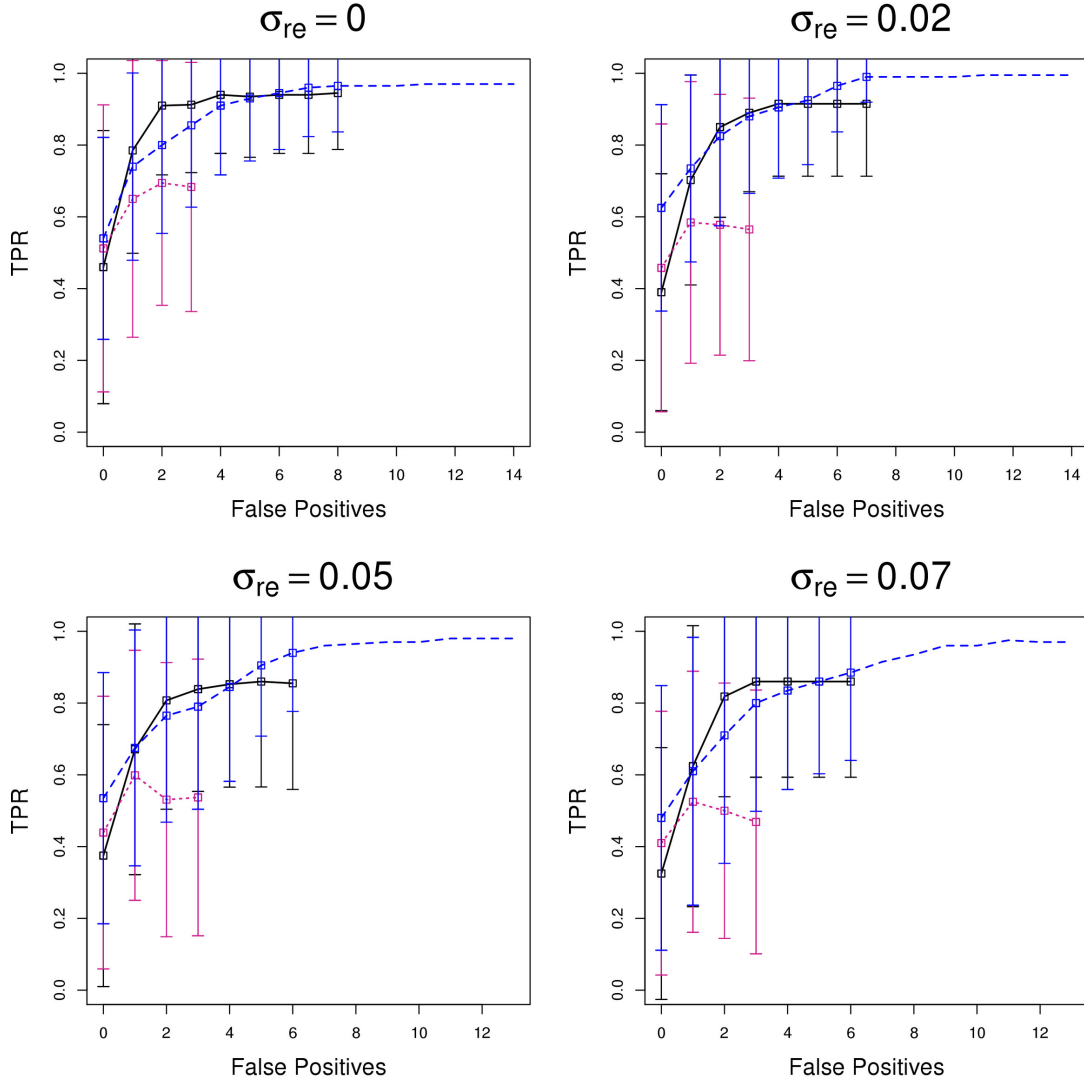

Fig. 4: Performance of JADE and competing methods in the binomial simulations presented in Figure 5 of the main text. Here, performance is quantified using a region-level analysis, described in Section E.2. Methods shown are JADE (—), methylKit (---), and BSmooth (---). Additional details are as in Supplementary Figure 2.

and Puri, 2006; Carrió and others, 2015). Here we assess whether the DMRs detected by JADE in Section 5 are consistent with this expectation.

Each DMR detected by JADE induces some ordering in the estimated mean profiles. For

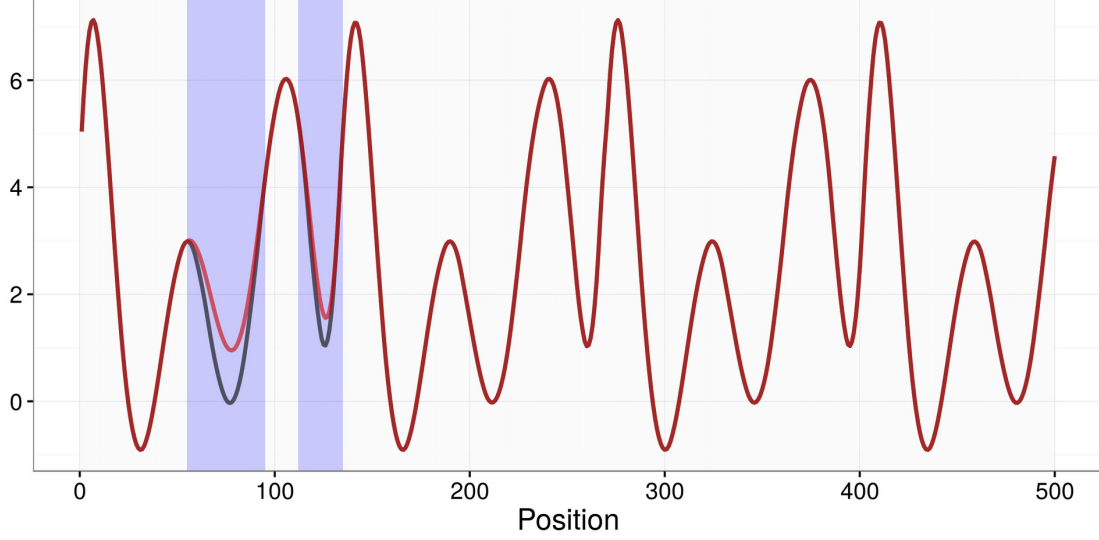

Fig. 5: Mean profiles for more challenging simulation setting described in Section E.2.

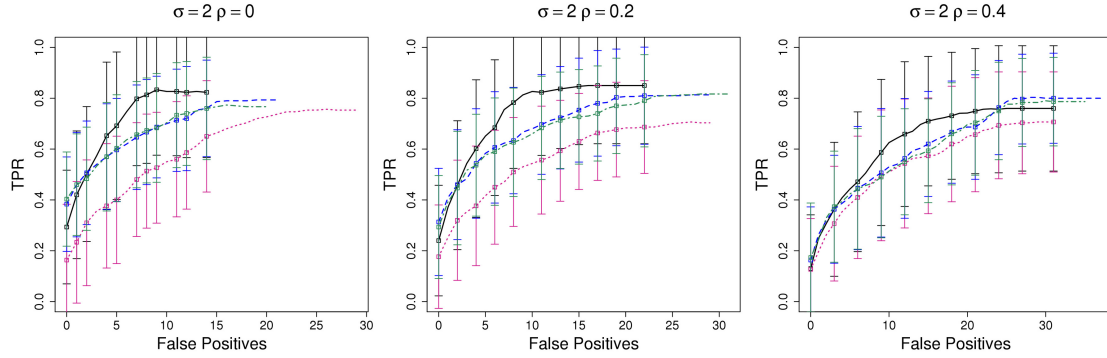

Fig. 6: Performance of JADE and competing methods in the more challenging simulation setting described in Section E.2, with mean profiles given in Supplementary Figure 5. Additional details are as in Supplementary Figure 2.

instance, the differential region shown on the left-hand side of Figure 6b in the main text has the ordering (Mature<Myoblast<Myotube), and the differential region shown on the right-hand side of Figure 6b in the main text has the ordering (Mature<Myoblast=Myotube).

We will refer to a DMR with the induced ordering (Mature $\leq$ Myotube $\leq$ Myoblast) as a “loss-of-methylation” DMR, as such a DMR displays a monotone decrease in methylation over the course of development. We will refer to a DMR with the induced ordering (Mature $\geq$ Myotube $\geq$ Myoblast)

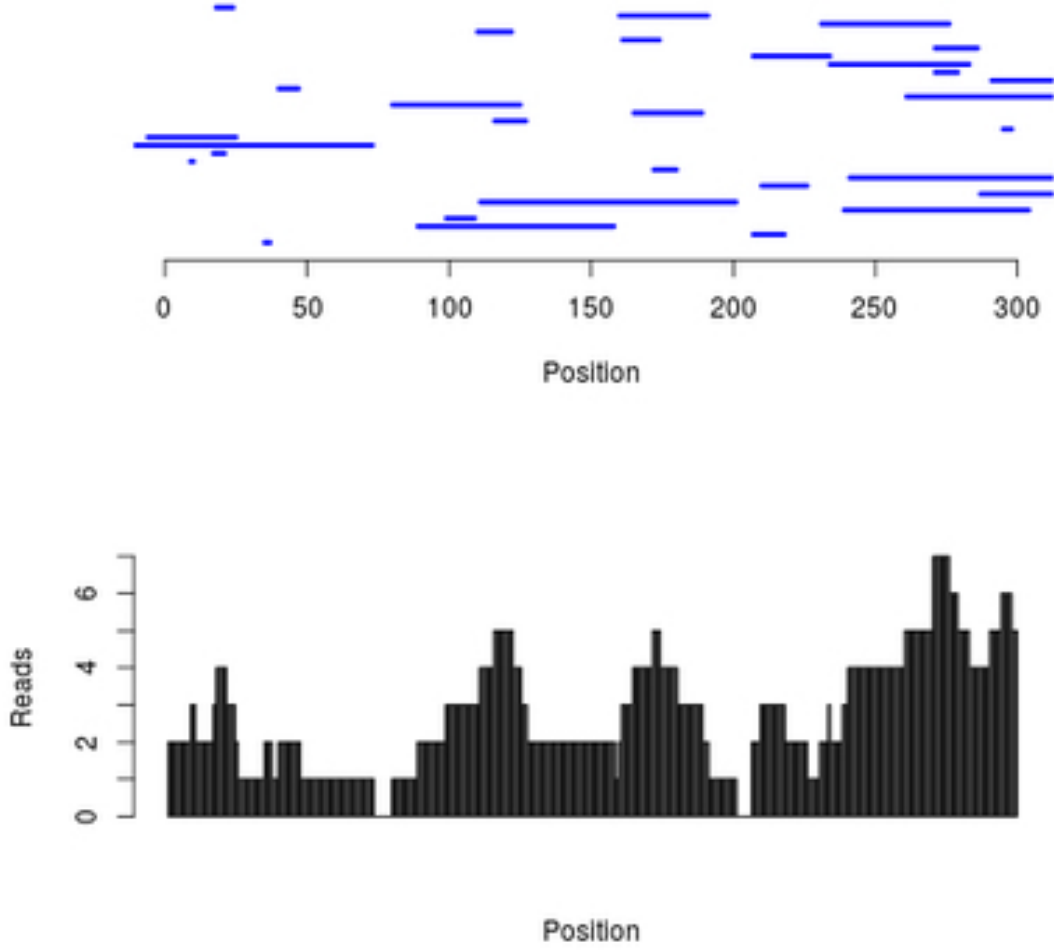

Fig. 7: Read tiling for binomial simulations in Section 4.2. The tiling procedure is described in Section F. *Top panel:* Read tiles. *Bottom Panel:* Total reads.

as a “gain-of-methylation” DMR. Some DMRs display neither loss-of-methylation nor gain-of-methylation over the course of development. For instance, the DMR shown on the left-hand side of Figure 6b of the main text is disordered with respect to developmental stage.

The orderings induced by the DMRs detected by JADE are summarized in Supplementary

Figure 8. Of the base-pairs that belong to a DMR, 35.9% fall within a loss-of-methylation DMR, 21.9% fall within a gain-of-methylation DMR, and the remaining 42.2% are disordered with respect to developmental stage. Of the DMRs that are disordered with respect to developmental stage, 94% have the ordering (Mature<Myoblast<Myotube) or (Myotube<Myoblast<Mature), and many of these display very small differences between the myoblast and myotube profiles, and much larger differences between the mature cell profiles and the other two. This makes them very similar to the classes (Mature<Myoblast=Myotube) and (Myotube=Myoblast<Mature), which are consistent with loss-of-methylation and gain-of-methylation, respectively.

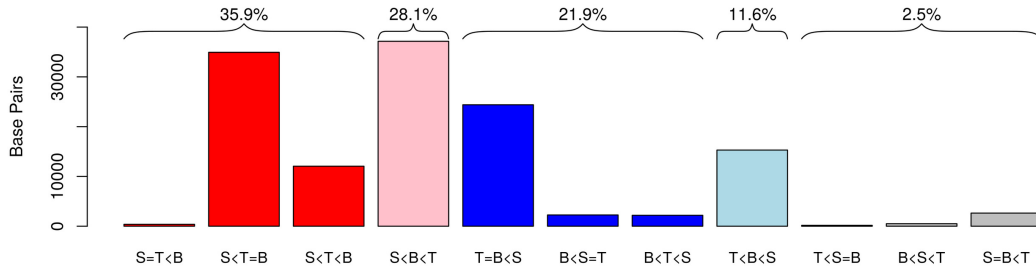

Fig. 8: Results from the methylation data analysis, as described in Section G.1. Each  $x$ -axis label indicates an ordering of the mean methylation profiles. For instance,  $S=T<B$  indicates the set of DMR sub-regions for which the estimated mean mature skeletal muscle profile (S) equals the estimated mean myotube profile (T), and is less than the estimated mean myoblast profile (B). For DMR sub-regions in which the estimated mean profiles for two tissue types intersect, the order is determined based on the average difference between profiles. The  $y$ -axis represents the total base-pairs in the DMR sub-regions with the specified ordering. Red bars are consistent with a decrease in methylation over the course of development, and bright blue bars are consistent with an increase in methylation over development. The proportion of total base-pairs in DMRs accounted for by each category is indicated.

## G.2 Enrichment Analysis of DMRs

In order to assess the quality of the DMRs detected by JADE, in Section 5.2.2, we test the hypothesis that these DMRs overlap genetic features no more than expected due to chance. The

Genomic Association Test (GAT; [Heger and others, 2013](#)) provides one approach for testing this hypothesis. However, this approach does not account for the possibility that the JADE output may depend on aspects of the data such as measurement density, read depth, or average methylation, which might also be correlated with genetic features of interest.

Instead, we conducted three “null” analyses, one for each cell type. In each of these analyses, we applied JADE to the data from a single cell type, treating each technical replicate as a separate group. The segments detected in these null analyses can be used to estimate the amount of overlap with a genetic feature that one might expect due to chance. We combined the three sets of “null” DMRs detected across the three cell types, and used a Fisher’s exact test to compare the proportion of detected DMRs overlapping each genetic feature to the proportion observed in the null analyses. These results are shown in Table 1 of the main text.

In addition, we tested whether each genetic feature has a tendency to overlap gain-of-methylation DMR sub-regions, or a tendency to overlap loss-of-methylation DMR sub-regions. (Recall that loss-of-methylation and gain-of-methylation DMR sub-regions are defined in Section Section G.1 of the SM.) Table 1 of the SM displays the results of this analysis. As discussed in the main text, we found that the rate of overlap with CpG islands is higher in loss-of-methylation than in gain-of-methylation DMR sub-regions and that the rates of overlap with both DNase-I hypersensitive sites and H3K27ac modifications are higher in gain-of-methylation than in loss-of-methylation DMR sub-regions.

Table 1: Overlap between gain-of-methylation and loss-of-methylation DMR sub-regions and genetic features, for the methylation data analysis described in Section 5.2.2 of the main text. ‘Total’, ‘Loss’, and ‘Gain’ are the number of DMR sub-regions, loss-of-methylation DMR sub-regions, and gain-of-methylation DMR sub-regions that overlap each genetic feature. ‘P-value’ is the  $p$ -value based on a Fisher’s exact test comparing whether the proportion of loss-of-methylation DMRs overlapping a genetic feature equals the proportion of gain-of-methylation DMRs overlapping the genetic feature. Note that the counts in the ‘Total’ column differ from those in Table 1 of the main text because here we are considering sub-regions rather than full DMRs. Furthermore, the ‘Loss’ and ‘Gain’ columns do not sum to equal the ‘Total’ column because only 58% of DMR sub-regions can be characterized as either loss-of-methylation or gain-of-methylation.

| Genetic Feature           | Total (N=380) | Loss (N=176) | Gain (N=46) | P-Value             |
|---------------------------|---------------|--------------|-------------|---------------------|
| CpG Islands               | 201 (52.9%)   | 100 (56.8%)  | 12 (26.1%)  | $2.3 \cdot 10^{-4}$ |
| CpG Island Shores         | 89 (23.4%)    | 36 (20.5%)   | 14 (30.4%)  | 0.17                |
| Transcription Start Sites | 186 (48.9%)   | 82 (46.6%)   | 23 (50%)    | 0.74                |
| TF Binding Sites          | 24 (6.3%)     | 13 (7.4%)    | 6 (13%)     | 0.24                |
| DNase I HS Sites          | 120 (31.6%)   | 52 (29.5%)   | 22 (47.8%)  | 0.022               |
| H3K27ac Modifications     | 43 (11.3%)    | 18 (10.2%)   | 10 (21.7%)  | 0.046               |

## REFERENCES

- BOYD, STEPHEN, PARIKH, NEAL, CHU, ERIC, PELEATO, BORJA AND ECKSTEIN, JONATHON. (2010). Distributed Optimization and Statistical Learning via the Alternating Direction Method of Multipliers. *Foundations and Trends in Machine Learning* **3**(1), 1–122.
- CARRIÓ, ELVIRA, DÍEZ-VILLANUEVA, ANNA, LOIS, SERGI, MALLONA, IZASKUN, CASES, ILDEFONSO, FORN, MARTA, PEINADO, MIGUEL A. AND SUELVES, MÒNICA. (2015). Deconstruction of DNA Methylation Patterns During Myogenesis Reveals Specific Epigenetic Events in the Establishment of the Skeletal Muscle Lineage. *Stem Cells* **33**(6), 2025–2036.
- DANAHER, PATRICK, WANG, PEI AND WITTEN, DANIELA M. (2014). The joint graphical lasso for inverse covariance estimation across multiple classes. *Journal of the Royal Statistical Society. Series B: Statistical Methodology* **76**(2), 373–397.
- HEGER, ANDREAS, WEBBER, CALEB, GOODSON, MARTIN, PONTING, CHRIS P. AND LUNTER, GERTON. (2013, aug). GAT: A simulation framework for testing the association of genomic intervals. *Bioinformatics* **29**(16), 2046–2048.
- HUPKES, M., JONSSON, M. K. B., SCHEENEN, W. J., VAN ROTTERDAM, W., SOTOGA, A. M., VAN SOMEREN, E. P., VAN DER HEYDEN, M. A. G., VAN VEEN, T. A., VAN RAVESTEIN-VAN OS, R. I., BAUERSCHMIDT, S., PIEK, E., YPEY, D. L., VAN ZOELLEN, E. J. *and others*. (2011, nov). Epigenetics: DNA demethylation promotes skeletal myotube maturation. *The FASEB Journal* **25**(11), 3861–3872.
- PALACIOS, DANIELA AND PURI, PIER LORENZO. (2006, apr). The epigenetic network regulating muscle development and regeneration. *Journal of Cellular Physiology* **207**(1), 1–11.
- RAMDAS, AADITYA AND TIBSHIRANI, RYAN J. (2015, jun). Fast and Flexible ADMM Algorithms for Trend Filtering. *Journal of Computational and Graphical Statistics*.

- SEGALÉS, JESSICA, PERDIGUERO, EUSEBIO AND MUÑOZ-CÁNOVES, PURA. (2014, sep). Epigenetic control of adult skeletal muscle stem cell functions. *FEBS Journal* **282**(9), 1571–1588.
- TIBSHIRANI, ROBERT, SAUNDERS, MICHAEL, ROSSET, SAHARON, ZHU, JI AND KNIGHT, KEITH. (2005, feb). Sparsity and smoothness via the fused lasso. *Journal of the Royal Statistical Society. Series B: Statistical Methodology* **67**(1), 91–108.
- TIBSHIRANI, RYAN J. (2014, feb). Adaptive piecewise polynomial estimation via trend filtering. *The Annals of Statistics* **42**(1), 285–323.
